# Supplementary material for: Image Quality Assessment for Magnetic Resonance Imaging
Source: arXiv:2203.07809 source file (2022-07-01)
Supplement: Supplementary file 1 [file iqa_datasets.tex]

\section*{IQA datasets}
\label{sec:iqa-datasets}

% Overview of datasets, may be should be moved to the dedicated Dataset selection section
Most of research relies on existing IQA databases.
However, in some cases, along with the work on extensive evaluation of existing methods, authors also provide new datasets.
These datasets are typically designed to evaluate existing IQMs on their ability to answer previously not considered questions such as IQA from two different view distances (CID dataset \cite{Pedersen2015}), IQA on images perturbed with multiple types of distortions (MDID \cite{sun2017mdid}, MD-IVL \cite{corchs2017multidistortion} and VLC \cite{Zaric2011vcl} datasets), evaluation of GAN-based image restoration algorithms (PIPAL \cite{Jinjin2020pipal} and NTIRE 2021 \cite{Gu2021ntire} challenges and datasets).
Another commonly used datasets are LIVE \cite{LIVE_MD}, TID2013 \cite{TID2013} and KADID-10k \cite{kadid10k}. 
Some works even try to propose a method to construct a general-case IQA dataset with extremely diverse image characteristics to evaluate \cite{Lin2018kaniq10k}.

% About structure of datasets
Majority of the listed datasets provide image pairs accompanied with subjective quality scores.
Typically, subjective scores are estimated by human assessors and aggregated in the form of Mean Opinion Scores (MOS) or Differential Mean Opinion Scores (DMOS).

\subsection{Database selection}
A significant number of IQA databases have come out over the last 15 years. 
There is currently no \textit{gold standard} dataset. 
As can be seen in Table \ref{table:iqa_datasets}, IQA datasets use a variety of subjective testing methodologies, number of images and number of distortions. 
Their benchmark quality ratings have different ranges and are either in the form of Difference Mean Opinion Scores (DMOS) or Mean Opinion Scores (MOS).

\begin{table}[tbh!]
\caption{Overview of existing IQA datasets}
\vspace{3mm}
\setlength\tabcolsep{2.5pt}
\begin{center}
\resizebox{1\columnwidth}{!}{ 
\begin{tabular}{c|cccc}
\toprule

Database &Year & Reference & Distorted & Subjective Score\\
\midrule

IVC \cite{le2005subjective} & 2005 & 10 & 235 & MOS (1 $\sim$ 5)\\
LIVE IQA \cite{sheikh2006statistical, LIVE_R2} & 2006 & 29 & 779 & DMOS (0 $\sim$ 100) \\ 
A57 \cite{chandler2007a57, chandler2007vsnr} & 2007 & 3 & 54 & DMOS (0 $\sim$ 1) \\
Toyama/MICT \cite{horita2011mict} & 2008 & 14 & 168 & MOS (1 $\sim$ 5)\\
TID2008 \cite{ponomarenko2009tid2008} & 2008 & 25 & 1700 & MOS (0 $\sim$ 9)\\
CSIQ \cite{larson2010most, CSIQ} & 2009 & 30 & 866 & DMOS (0 $\sim$ 1) \\
% BID & - & - & 585 \\
% MDIQ & 15 & 405\\
IVC-LAR \cite{Strauss2009ivclar} & 2009 & 8 & 120 & MOS (1 $\sim$ 5)\\
WIQ \cite{2009wiq_dataset} & 2009 & 7 & 80 & DMOS (0 $\sim$ 100)\\
IRSQ \cite{Ma2012irsq} & 2012 & 57 & 171 & MOS (0 $\sim$ 5)\\
VCLFER \cite{zaric2012vcl, VCLFER} & 2012 & 23 & 552 & MOS (0 $\sim$ 100)\\
LIVE MD \cite{jayaraman2012objective, LIVE_MD} & 2013 & 15 & 405 & DMOS (0 $\sim$ 100) \\
TID2013 \cite{ponomarenko2015image, TID2013} & 2013 & 25 & 3000 & MOS (0 $\sim$ 9)\\
MDID2013 \cite{gu2014hybrid} & 2014 & 12 & 324 & DMOS (0.3 $\sim$ 0.6) \\
CID2013 \cite{virtanen2015cid2013} & 2013 & 8 & 480 & MOS (0 $\sim$ 9)\\
CIDIQ \cite{Liu2014CIDIQ} & 2014 & 23 & 690 & MOS (0 $\sim$ 9)\\
SIQAD \cite{yang2015perceptual} & 2015 & 20 & 980 & DMOS (0 $\sim$ 100) \\
LIVE in the wild \cite{Ghadiyaram2016livewild1, Ghadiyaram2016livewild2} & 2016 & - & 1162 & MOS (1 $\sim$ 5)\\
MD-IVL \cite{corchs2017multidistortion, MD-IVL} & 2017 & 10 & 750 & MOS (0 $\sim$ 100)\\
MDID \cite{sun2017mdid} & 2017 & 20 & 1600 & MOS (0 $\sim$ 9)\\
% % KonIQ-10k & 2018\\
KADID-10k \cite{kadid10k} & 2019 & 81 & 10125 & MOS (1 $\sim$ 5) \\
\bottomrule
\end{tabular}
}
\end{center}
% \vspace{-3mm}
\label{table:iqa_datasets}
% \vspace{-8mm}
\end{table}

Due to small number of images and distortions, result may varies widely across different datasets. 
Considering that, our main criterion for selection were size of dataset and distortions variety. 
As can be seen next, with enough images results are more consistent. 

TID2013 \cite{TID2013} and KADID-10k \cite{kadid10k} databases were selected. 

\subsection{Implementation details}
Selected IQAs were re-implemented in PyTorch, rigorously tested and collected in the PyTorch Image Quality library \cite{piq}. 
New implementations are verified to produce virtually the same correlation scores on TID2013 \cite{TID2013}, KADID-10k \cite{kadid10k} and PIPAL \cite{Jinjin2020pipal} datasets.
In case if there are official Python or MATLAB implementations, it is checked that results produced by new implementations differ no more than on a computational error.

Most of the above mentioned metrics require full images normalized into $[0, 1]$ before score computation. 
We applied sigmoid function after raw model outputs to keep all values in a given range. 
After that, we computed FR, NR and DB IQMs. 
Note that DB metrics are not originally designed for pair-wise comparison of images. 
Instead, they are intended to be used to compare distributions of two image sets.
In our study we investigate DB metrics for pair-wise comparison of images.
To encounter for the initial setting, we represent each image in a pair as a set of overlapping patches of size $96 \times 96$, which allows us to reformulate pair-wise comparison of images as comparison of distributions of patches.
The same approach is used later for medical data evaluation.

\subsection{Evaluation}

\subsubsection{Pearson Linear Correlation Coefficient (PLCC)}

This criteria requires produced scores to be linear with respect to subjective ratings. 
A common solution is applying a nonlinear regression. 
We do this by adopting the five-parameter modified logistic function used in \cite{sheikh2006statistical}.

$$
P(Q) = \beta_1 \cdot \left(\frac{1}{2} - \frac{1}{1 + \textrm{exp}(\beta_2 \cdot (Q - \beta_3))} \right) + \beta_4 \cdot Q + \beta_5
$$

where Q denotes the objective quality scores directly from an IQA method, P denotes the IQA scores after the regression step, and $\beta_1$, $\beta_2$, $beta_3$, $\beta_4$ and $\beta_5$ are model parameters that are found numerically to maximize the Mean Squared Difference between subjective and objective scores. 

The Pearson Linear Correlation Coefficient is often used as a measure of a method’s prediction accuracy [53]. 

Given a database with its subjective scores denoted by S, the PLCC value of an IQA method is then calculated as:

$$
\text{PLCC} (P, S) = \frac{\sum_{i=1}^{N} (P_i - \overline{P}) \cdot (S_i - \overline{S})}{\sqrt{\sum_{i=1}^{N} (P_i - \overline{P})^2 \cdot \sum_{i=1}^{N} (S_i - \overline{S})^2}}
$$

%  \subsubsection{Root Mean Square Error}
% Another metric commonly to measure IQA methods is root-mean-squared-error (RMSE) between DMOS and the algorithm score after nonlinear regression. It showed to be very consistent with PLCC and less informative, so it's not evaluated in this study. 
 
%  $$
% \text{RMSE} = \sqrt{ \frac{1}{N} \sum_{i=1}^{N} (P_i - S_i)^2}
% $$

\subsubsection{Spearman Rank-order Correlation Coefficient}

Prediction monotonicity is measured using the Spearman rank-order correlation coefficient (SRCC). SRCC is a non-parametric rank-order based correlation metric and does not require the preceding nonlinear mapping step \cite{sheikh2006statistical}. The SRCC value of an IQA method on a database with N images is calculated as:

$$
\text{SRCC} (Q, S) = 1 -  \frac{6 \sum_{i=1}^{N} d_i ^ 2}{N (N^2 - 1)},
$$
\noindent
where $d_i$ is the difference between the \textit{i}-th image’s ranks in the objective (Q) and subjective (S) scores.

\subsubsection{Kendall’s Rank-order Correlation Coefficient}

KRCC is found to be highly consistent with the SRCC\cite{athar2019comprehensive}, but anyway still reported in this paper.

Kendall rank correlation is used to test the similarities in the ordering of data when it is ranked by quantities. Other types of correlation coefficients use the observations as the basis of the correlation, Kendall’s correlation coefficient uses pairs of observations and determines the strength of association based on the patter on concordance and discordance between the pairs.

$$
\tau= \frac{2}{n(n-1)}\sum_{i<j} \text{sign}(x_i-x_j)\;\text{sign}(y_i-y_j)
$$

\begin{table}[tbh!]
\caption{Comparison of metrics performance on MOS datasets. \\
Top-4 performers in each category are marked in bold. \\$^*$ denotes values taken directly from \cite{Golestaneh2021noreferencereview}}
\vspace{3mm}
\setlength\tabcolsep{2.5pt}
\begin{center}
\resizebox{.8\columnwidth}{!}{ 
\begin{tabular}{lccccc}
\toprule

&\multicolumn{2}{c}{TID2013}&&\multicolumn{2}{c}{KADID-10k}  \\
 \cmidrule{2-3} \cmidrule{5-6}
 & SRCC & KRCC && SRCC & KRCC \\
  \cmidrule{1-6}
  PSNR & $0.69$ & $0.50$ && $0.68$ & $0.49$\\
  SSIM \cite{wang2004image} & $0.55$ & $0.39$ && $0.63$ & $0.46$\\
  MS-SSIM \cite{wang2003multiscale} & $0.80$ & $0.60$ && $0.80$ & $0.61$\\
  IW-SSIM \cite{wang2010information} &  $0.78$ &  $0.60$ && $0.85$ & $0.67$\\
  VIFp \cite{sheikh2005visual} & $0.46$ & $0.32$ && $0.67$ & $0.50$\\
  GMSD \cite{xue2013gradient} & $0.80$ & $0.63$ && $0.85$ & $0.66$\\
  MS-GMSD \cite{Zhang2017gmsd} & $0.81$ & $0.64$ && $0.85$ & $0.67$\\
  MS-GMSDc \cite{Zhang2017gmsd} & $\mathbf{0.89}$ & $\mathbf{0.71}$ && $\mathbf{0.87}$ & $\mathbf{0.69}$\\
  FSIM \cite{zhang2011fsim} & $0.80$ & $0.63$ && $0.84$ & $0.64$\\
  FSIMc \cite{zhang2011fsim} & $0.85$ & $0.67$ && $0.85$ & $0.66$\\
  VSI \cite{zhang2014vsi} & $\mathbf{0.89}$ & $\mathbf{0.72}$ && $\mathbf{0.88}$ & $\mathbf{0.69}$\\
  MDSI \cite{nafchi2016mdsi} & $\mathbf{0.89}$ & $\mathbf{0.71}$ && $\mathbf{0.89}$ & $\mathbf{0.70}$\\
  HaarPSI \cite{Reisenhofer2018haarpsi} & $\mathbf{0.87}$ & $\mathbf{0.70}$ && $\mathbf{0.88}$ & $\mathbf{0.70}$ \\
  Content\textsubscript{VGG16} \cite{johnson2016perceptual} & $0.67$ & $0.50$ && $0.71$ & $0.52$\\
  Style\textsubscript{VGG16} \cite{johnson2016perceptual} & $0.50$ & $0.35$ && $0.56$ & $0.40$\\
  LPIPS\textsubscript{VGG16} \cite{zhang2018unreasonable} & $0.67$ & $0.50 $ && $0.78$ & $0.52$\\ 
  DISTS \cite{ding2020image} & $0.71$ & $0.53$ && $0.81$ & $0.62$\\
  PieAPP \cite{Prashnani2018pieapp} & $0.84$ & $0.65$ && $\mathbf{0.87}$ & $0.68$\\
  DSS \cite{Balanov2015dss} & $0.79$ & $0.61$ && $0.86$ & $0.67$ \\
  \cmidrule{1-6}
\multicolumn{6}{c}{No-reference metrics} \\
\cmidrule{1-6}
  BRISQUE \cite{mittal2012no} & $0.20$ & $0.14$ && $0.20$ & $0.14$\\
  PaQ-2-PiQ \cite{paq2piq2020} & $0.86^*$ & $-$ && $0.84^*$ & $-$ \\
  MetaIQA \cite{MetaIQA2020} & $0.86^*$ & $-$ && $0.76^*$ & $-$ \\

  \cmidrule{1-6}
\multicolumn{6}{c}{Distribution-based metrics} \\
\cmidrule{1-6}
  KID\textsubscript{InceptionV3} \cite{binkowski2018demystifying} & $0.42$ & $0.31$ && $0.63$ & $0.46$\\
  FID\textsubscript{InceptionV3} \cite{heusel2017gans} & $0.67 $ & $0.50$ && $0.66$ & $0.49$\\
  GS\textsubscript{InceptionV3} \cite{khrulkov2018geometry} & $0.37$ & $0.26$ && $0.37$ & $0.26$\\
  IS\textsubscript{InceptionV3} \cite{salimans2016improved} & $0.26$ & $0.18$ && $0.25$ & $0.19$\\
  MSID\textsubscript{InceptionV3} \cite{tsitsulin2020shape} & $0.21$ & $0.14$ && $0.32$ & $0.22$ \\
  
  KID\textsubscript{VGG16} \cite{binkowski2018demystifying} & $0.70$ & $0.52$ && $0.71$ & $0.53$\\
  FID\textsubscript{VGG16} \cite{heusel2017gans} & $0.74$ & $0.55$ && $0.70$ & $0.52$\\
  GS\textsubscript{VGG16} \cite{khrulkov2018geometry} & $0.47$ & $0.33$ && $0.45$ & $0.32$\\
  IS\textsubscript{VGG16} \cite{salimans2016improved} & $0.64$ & $0.46$ && $0.65$ & $0.42$\\
  MSID\textsubscript{VGG16} \cite{tsitsulin2020shape} & $0.69$ & $0.51 $ && $0.64$ & $0.46$\\
  
  KID\textsubscript{VGG19} \cite{binkowski2018demystifying} & $0.54$ & $0.37$ && $0.59$ & $0.42$ \\
  FID\textsubscript{VGG19} \cite{heusel2017gans} & $0.68$ & $0.48$ && $0.75$ & $0.55$\\
  GS\textsubscript{InceptionV3} \cite{khrulkov2018geometry} & $0.35$ & $0.24$ && $0.41$ & $0.29$\\
  IS\textsubscript{InceptionV3} \cite{salimans2016improved} & $0.28$ & $0.19$ && $0.33$ & $0.24$\\
  MSID\textsubscript{InceptionV3} \cite{tsitsulin2020shape} & $0.11$ & $0.08$ && $0.13$ & $0.09$ \\

\bottomrule
\end{tabular}
}
\end{center}
% \vspace{-3mm}
\label{table:metrics-comparison}
% \vspace{-8mm}
\end{table}

\subsection{Results}

Aggregated scores for all metrics and datasets can be seen in Table
\ref{table:metrics-comparison}. 

\subsection{Model evaluation}

We conducted a @ alternative forced choice study to compare metrics with each other.

11 people took part in the labeling experiment, which produced nearly 1800 labels, 7-8 labels per image.

% \subsection{Rank aggregation}

% % Здесь рассказать о том, как мы перешли от результов парных сравнений к итоговым оценкам метрик. 

% \section{Algorithms}
% \label{algorithms}

% \section{Models}
% \label{models}
% For qualitative assessment of the results we used 2 different models, which are described in details below. The reason we took those architectures is that the are well-known and used in lot's for comparison in lot's of modern papers. So the results we get can be easily compared with others. 

% See table \ref{table:metrics_comparison}

\subsubsection{DnCNN}
First proposed in \cite{zhang2017beyond} this model is a simple feed-forward convolutional network which can be used to learn the residual mapping between distorted input image and target. Main building block of this model consists of  Convolution - Batch-Normalization - Activation. Those buildings blocks can be stacked to get model of arbitrary depth $D$.

\subsubsection{UNet}
This model was initially used for solving task of semantic segmentation \cite{ronneberger2015u}, but later can be also used for denosing, super-resolution and debluring. 
Update

Despite it's effiency, UNet models are well-know for produsing checker board artefacts due to bad combination of kernel size and output stride in Deconvolution layer. To avoid this, we changed the upsamling method to recently proposed PixelShuffle technique.

\subsection{Subjective testing}

We conducted a subjective study to collect human opinions on the perceptual quality of selected models. To allow differentiation of fine-grained quality variations, we employed a 2-alternative forced choice (2AFC) method. Subjects were asked to choose which of two images has better perceived quality, the original image was not shown. We formed a total of $\binom{5}{2} \times 3 \times 10 = 300$ pairs and removed comparisons made with identical models. This resulted in $178$ pairs.

Our customized graphical user interface also allows them to zoom in/out any portion of the two images for a more careful visual comparison. A two-alternative forced choice (2AFC) method was employed, allowing differentiation of fine-grained quality variations. Specifically, subjects were asked to choose which of two images has better perceived quality. The original image was also shown for reference. Subjects were allowed unlimited viewing time, and were free
