# Supplementary material for: Image Quality Assessment for Magnetic Resonance Imaging
Source: arXiv:2203.07809 source file (2022-07-01)
Supplement: Supplementary file 2 [file quality_metrics.tex]

\section*{Supplementary material}
\section*{Quality Metrics}
\label{sec:quality-metrics}

Depending on the availability of a reference image, which is presumed to be of perfect quality, all IQA metrics can be broadly classified into three major categories:
Full-Reference (FR), Fused Full-Reference (FFR), and No-Reference (NR). FR requires access to the reference image, FFR combines several FR methods, while NR metrics attempt to perform IQA without the reference. 

More detailed classification can be seen in Figure \ref{metrics_tree}.
\begin{figure*}[h]
\centering
  \includegraphics[width=0.75\textwidth]
    {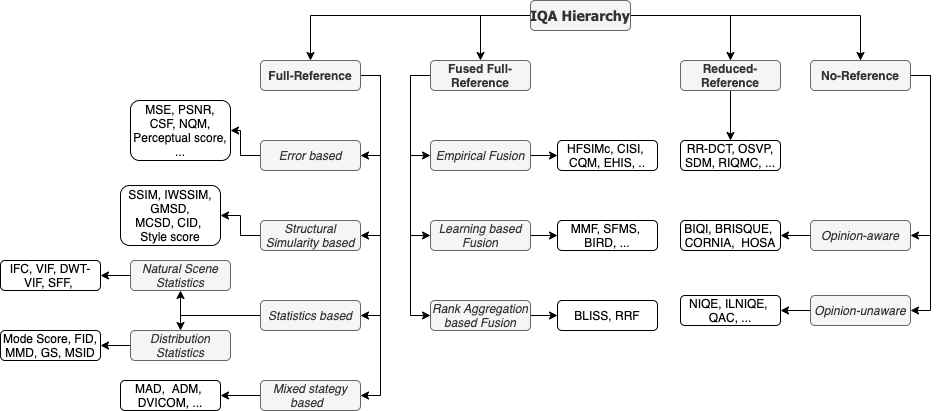}
  \caption{General taxonomy of IQA algorithms.}
  \label{metrics_tree}
\end{figure*}

% Most relevant for image transformation tasks are Full-Reference and No-Reference.
In our work, we choose to evaluate representative methods from those categories. A short description of the design philosophies is given in the following section.

\subsection*{Full-Reference}

Those methods evaluate the quality of a distorted image with respect to the corresponding original (reference) image assumed to be distortion-free and of pristine quality, \cite{sheikh2006statistical}. Only a subset of all existing metrics in analyzed due to their inheritance nature and clear domination of some of them over the others \cite{athar2019comprehensive}. We tried to represent different IQA design philosophies and take an example from each group.

\subsubsection*{Error Based Methods}

\begin{enumerate}
    \item Mean Squared Error (\textbf{MSE}) - is the most used quality metric \cite{wang2006modern}. It measures distance directly between pixels of distorted and reference image and provides many desirable properties \cite{wang2009mean}.
    
    \item Peak Signal-to-Noise Ratio (\textbf{PSNR}) - is closely related with MSE and de-facto standard way of measuring image quality \cite{wang2006modern}.  It is defined as a ratio between the maximum possible power of a signal and the power of corrupting noise that affects its representation's fidelity.
    
    \item Information Weighted PSNR (\textbf{IW-PSNR}) \cite{wang2010information} - uses information-theoretic principles to add more weight for regions of visual content which ix perceptually more important than others, either due to the visual attention property of the human visual system (HVS) or due to the influence of distortions.
    % compute information content weights, which are used in the pooling stage of quality score generation.  weightens 
    % underlying premise is that some  IW-PSNR uses information-theoretic principles to calculate information content weights used in the pooling stage of quality score generation. 
    
    \item Most Apparent Distortion (\textbf{MAD}) \cite{larson2010most} - explicitly models adaptive strategies of the human visual system (HVS). For high-quality images with only near-threshold distortions, a detection-based strategy is employed, and an appearance-based strategy is activated if the distortions are visible. 
    % Image quality is determined as the absolute difference between low-level statistics, including the mean, variance, skewness, and kurtosis, of the weighted coefficients. Based on the distortion amount, the detection and appearance quality scores are then combined through a weighted geometric mean to give the final MAD score.

    \item Content Score often referred to as VGG loss, \cite{johnson2016perceptual} - computes the distance between features of distorted and reference images taken from some convolutional neural network (CNN), mainly of the VGG family. 
    
    \item Style score \cite{johnson2016perceptual}  - extracts and compares texture information from the images by computing Gram matrixes between features from CNN and taking MSE between them.
    
    \item Learned Perceptual Image Patch Similarity (\textbf{LPIPS}) \cite{zhang2018unreasonable} - takes a step further and learns weights for different layers of the VGG network, building on the premise that different layers represent different structures on the image
    
\end{enumerate}

\subsubsection*{Structural Simularity Based Methods}
The difference concerning other methods mentioned earlier, such as PSNR or Content score, is that they estimate absolute errors; on the other hand, the structural similarity is a perception-based model that considers image degradation as perceived change in structural information also including luminance and contrast masking terms. These methods are based on the idea that pixels have strong inter-dependencies, especially when they are spatially close. 
% These are constructed to measure the similarity of local image “structures.”

\begin{enumerate}
    \item Structural Similarity Index Measure (\textbf{SSIM}) \cite{wang2004image, wang2006modern} - it has become a de-facto standard in the field of perceptual image processing and has inspired subsequent IQA models based on feature similarity \cite{wang2003multiscale}. SSIM  operates in the spatial domain and performs three types of comparisons between the reference and distorted images: luminance, contrast, and structure. 
    
    % Luminance comparison is a function of the mean intensity of the images being compared, while contrast comparison is a function of standard deviations. Structural comparison is made by comparing the image patches being compared after mean subtraction and variance normalization. 
    All comparisons are made locally by a sliding window, and the three SSIM components are combined, leading to local quality scores, which lead to a quality map. 
    % The overall quality score for the entire distorted image with respect to the reference image is obtained by taking the mean of all the local quality scores. 
    
    \item Multi-scale SSIM (\textbf{MS-SSIM} \cite{wang2003multiscale} - accounts for the variations in viewing conditions by measuring SSIM on 5 different scales. Contrast and structure similarities are measured on all scales, while luminance comparison occurs only at the final scale. Scores then combined through a weighted product using weights adjusted on the human opinions dataset. 
    
    % comparisons are performed at all scales, while the luminance comparison takes place only at the final scale. The quality scores obtained at each scale are combined through a weighted product. The weights assigned to different scales are obtained through an image synthesis calibration experiment that involved subjective testing.
    
    \item Information Weightened SSIM (\textbf{IW-SSIM}\cite{wang2010information} - operates at five scales, as MS-SSIM, and uses information-theoretic principles to compute information content weights that are used in the pooling stage. 
    
    \item Feature Similarity Index Measure (\textbf{FSIM}) \cite{zhang2011fsim} - uses phase congruency and gradient magnitude maps as the primary features to evaluate image similarity, which is then combined through a weighted product. A color-sensitive version of FSIM, called FSIMc \cite{zhang2011fsim} first converts RGB images into YIQ color space and then computes FSIM on luminance channel and chrominance similarity maps on I and Q channels.
    
    % Since phase congruency is contrast invariant, and the gradient magnitude is used as a secondary feature in FSIM to capture contrast information. The phase congruency and gradient magnitude maps of the reference and distorted images are compared, leading to phase congruency and gradient magnitude quality maps, which are then combined into a single quality map for the luminance channel of the images through a weighted product. The final FSIM quality score is obtained by pooling this quality map using a weighting function derived from the phase congruency maps of the images being compared. The color version of FSIM, called FSIMc \cite{zhang2011fsim}, converts RGB images into YIQ color space and then computes FSIM on luminance channel and chrominance similarity maps on I and Q channels.
    
    % \item Gradient Similarity Measure(\textbf{GSM}) \cite{gsm_measure} - 
    % A Gradient Similarity-based IQA method (GSIM) is proposed in [85], where changes in contrast and structure in images being compared are measured through gradient comparison. It also takes into account masking effects, visibility threshold, and luminance distortions. GSIM combines the measurement of luminance distortion and contrast-structure distortion adaptively to give a final quality score, where more weight is given to the latter. 
    
    \item Gradient Magnitude Similarity Deviation (\textbf{GMSD}) - based on the idea that the global variation of image local quality degradation can reflect its overall quality, authors proposed to compute the standard deviation of the gradient similarity map as IQA index.
    
    % A natural image generally has a variety of local structures in its scene. When an image is distorted, the different local structures will suffer various degradations in gradient magnitude. For example, the distortions introduced by JPEG2000 compression include blocking, ringing, blurring, etc. Blurring will cause less quality degradation in flat areas than in textured areas, while blocking will cause higher quality degradation in flat areas than in textured regions.

    \item Multi-scale GMSD (\textbf{MS-GMSD}) - accounts for the variations in viewing conditions by measuring GMSD on five different scales, similar to MS-SSIM. Chromatic version, named MS-GMSDc, additionally measures chrominance dissimilarity
    % but only at the smallest scale, because the spatial resolution to color stimulation is much lower than luminance for visual perception.
    
     \item Deep Image Structure and Texture Similarity (\textbf{DISTS}) - computes SSIM on a subset of feature maps from the VGG16 network and combines scores using learned weights.
 
\end{enumerate}

\subsubsection*{Natural Scene Statistics based}

These methods attempt to measure some approximation of the mutual information between the perceived reference and distorted images as an indication of perceptual image quality. Statistical modeling of the image source, the distortion process, and the HVS is critical in algorithm development. 

\begin{enumerate}
    \item Visual Information Fidelity (\textbf{VIF}) \cite{sheikh2005visual} - uses a Gaussian scale mixture to statistically model the wavelet coefficients of a steerable pyramid decomposition of an image \cite{simoncelli1992shiftable}. It then predicts the distorted image quality by quantifying the amount of preserved information from the reference image. Its spatial domain, named VIFp, computes fidelity on raw pixels. 

    % \item IFC 
    
    % \item QASD 
    
\end{enumerate}

\subsubsection*{Distribution Statistics based}

This class of methods came from generative model evaluation when a direct comparison is not possible, and only distance between model distributions can be measured. The first embed samples into a feature space given by a specific neural net and then use 

% IMPORTANT NOTE!
% a critical concern regarding many measures is that they are sensitive to the choice of the feature space (e.g., different CNNs) as well as the distance type ($L2$ or $L1$). 

% Generative models can be classified into two broad categories of explicit and implicit approaches. The former class assumes access to the model likelihood function, whereas the latter uses a sampling mechanism to generate data. Examples of explicit models are variational auto-encoders (VAEs). Examples of implicit generative models are GANs. Explicit models are typically trained by maximizing the likelihood of its lower bound. GANs aim to approximate a data distribution $P$, using a parameterized model distribution $Q$. The main goal of distribution-based methods is to measure the distance between $P$ and $Q$ using a limited amount of samples.

\begin{enumerate}

    \item Freshet Inception Distance (\textbf{FID}) \cite{heusel2017gans} - views the embeddings of both predicted and target data as a product of continuous multivariate Gaussian. The mean and covariance are estimated for both, and the Fréchet distance between these two Gaussians (a.k.a Wasserstein-2 distance)  is then used to quantify the quality of the generated sample.

    \item Kernel Inception Distance (\textbf{KID}) \cite{binkowski2018demystifying}, sometimes referred to as Maximum Mean Discrepancy (MMD) -  computes the dissimilarity between two probability distributions $P$ and $Q$ by measuring squared MMD for some fixed characteristic kernel function (e.g., Gaussian kernel).

    \item Multi-Scale Intrinsic Distance (\textbf{MSID}) \cite{tsitsulin2020shape} - develops an intrinsic and multi-scale method for characterizing and comparing data manifolds, using a lower-bound of the spectral Gromov-Wasserstein inter-manifold distance, which compares all data moments
    
    \item Geometry Score (\textbf{GS}) \cite{khrulkov2018geometry} - constructs a performance measure by comparing geometrical properties of the underlying data manifolds. In particular, topological approximation for computation of connected components ("holoes") in homology using witness complex \cite{de2004topological} is introduced.

\end{enumerate}

\subsection*{No-Reference}

No-Reference (NR) IQA methods evaluate a distorted image's quality in the absence of any reference information \cite{sheikh2006statistical}. Thus they are also referred to as blind IQA methods.

\begin{enumerate}
    \item Blind/Referenceless Image Spatial Quality Evaluator (\textbf{BRISQUE}) - operates on locally normalized luminance values in the spatial domain, called Mean Subtracted Contrast Normalized (MSCN) coefficients. Various features are extracted from the MSCN coefficients and their pairwise products, which are then used to estimate Generalized Gaussian Distribution (GGD) and  Asymmetric GGD parameters. SVR model is then used to learn to map features to a quality score. 

    % \item Codebook Representation for No-Reference Image Assessment (\textbf{CORNIA} \cite{ye2012unsupervised} - 
    
    % \item deeIQ
    
    \item Inception score (\textbf{IS}) \cite{salimans2016improved} - uses pre-trained InceptionNet model for feature extraction and captures properties of generated sample
    to capture properties of generated samples: diversity with respect to class labels and high classifiability.

    \item Improved Inception score (\textbf{IS'}) \cite{barratt2018note} - proposed different way of feature aggregation, which improved both calculation and interpretability of the Inception Score. 
    
\end{enumerate}
